# Supplementary material for: Management of the Correlations of Ultracold Bosons in Triple Wells
Source: arXiv:1802.02407 source file (2018-02-07)
Supplement: Supplementary file 1 [file S_Dutta_Manybody_Correlations_Suppl_Mat_2018.pdf]

# Supplemental Material: Management of Coherence of Ultracold Bosons in Triple Wells

Sunayana Dutta,[1] Marios C. Tsatsos,[2] Saurabh Basu,[1] and Axel U. J. Lode[3,4,*]

[1] *Department of Physics, Indian Institute of Technology Guwahati, Guwahati-781039, Assam, India*

[2] *São Carlos Institute of Physics, University of São Paulo, P.O. Box 369, 13560-970 São Carlos, São Paulo, Brazil.*

[3] *Wolfgang Pauli Institute c/o Faculty of Mathematics, University of Vienna, Oskar-Morgenstern Platz 1, 1090 Vienna, Austria*

[4] *Vienna Center for Quantum Science and Technology, Atominstitut, TU Wien, Stadionallee 2, 1020 Vienna, Austria*

(Dated: January 30, 2018)

* axel.lode@univie.ac.at

This Supplemental Material discusses the numerical method used in this work, the multiconfigurational time-dependent Hartree method for bosons (MCTDHB), and provides further analysis that generalizes our main results. Sec. S1 sketches MCTDHB, Sec. S2 presents a complementary analysis of the one-body correlation function, Sec. S3 provides convergence checks for our computations and Sec. S4 collects complementary results for bosons with long-range interactions in a tilted triple well.

## S1. THE MCTDHB METHOD

MCTDHB is an approach which optimizes variationally both its many-body basis and the expansion coefficients in that basis. This optimization is carried out without any constraints on the number of orbitals, geometry of trap, dimensionality or shape (functional form) of the interparticle interaction potential of the time-dependent many-boson system. The complete derivation of the equations of motion and also the details of the numerical implementation of MCTDHB are found in Refs. [1–3]. MCTDHB is a powerful, exact theory that can describe the time-evolution of condensed or fragmented states and correlation functions as well. It has, recently, explained experimental results of highly fluctuating quantum states of perturbed bosonic gases [4].

The starting point for the derivation of the MCTDHB equations of motion is a general many-body (MB) ansatz [Eq. (4)], the Schrödinger equation for many interacting particles and a time-dependent variational principle [5]. The time-dependent many-body Schrödinger equation that governs the time evolution of $N$ interacting bosons is given as

$$\hat{H}\Psi = i\frac{\partial \Psi}{\partial t}. \tag{1}$$

Here, $\hat{H}$ is the general Hamiltonian with one- and two-body terms,

$$\hat{H}(\mathbf{r}_1, \mathbf{r}_2, ..., \mathbf{r}_N) = \sum_{j=1}^{N} \hat{h}(\mathbf{r}_j) + \sum_{k>j=1}^{N} \hat{W}(\mathbf{r}_j - \mathbf{r}_k). \tag{2}$$

Here $\mathbf{r}_j$ represents the position of the $j^{th}$ boson and the term $\hat{h}$ is the single-particle Hamiltonian, $\hat{h}(x) = \hat{T}(x) + \hat{V}_{\text{trap}}(x)$. $\hat{T}(x)$ is the usual kinetic energy and the external potential is

$$V_{\text{trap}}(x) = -\alpha x + V_0 \sin^4(kx) + f_w(x). \tag{3}$$

The second term in Eq. (2), $\hat{W}(x_j - x_k)$ is the two-body interaction.

The ansatz assumed in MCTDHB for the many-boson wave function is

$$|\Psi(t)\rangle = \sum_{n} C_{\vec{n}}(t)|\vec{n};t\rangle. \tag{4}$$

Here, the summation runs over all possible configurations $\{\vec{n} = (n_1, ..., n_M)\}$, for which $\sum_i n_i = N$. Thus $N$ bosons are distributed over $M$ accessible orbitals. With the help of bosonic creation operators $\{\hat{a}_k^\dagger\}$ the time-dependent configurations can be written as

$$\begin{aligned} |\vec{n};t\rangle &= \frac{[a_1^\dagger(t)]^{n_1}[a_2^\dagger(t)]^{n_2}...[a_M^\dagger(t)]^{n_M}}{\sqrt{n_1!n_2!n_3!...n_M!}}|0\rangle \\ &\equiv |n_1, n_2, n_3, ...n_M;t\rangle, \end{aligned} \tag{5}$$

where, $|0\rangle$ is the vacuum. Since the permanents $|n_1, ..., n_M;t\rangle$ are a complete basis set of $N$-body Hilbert space for $M \to \infty$, the variational principle [5] guarantees that the solutions of the time-dependent many-body problem provided by the MCTDHB method gradually improve towards exactness when the number of considered creation operators $M$ in the ansatz, Eq. (4), is increased [6, 7].

The MCTDHB thus yields descriptions of many-boson systems that allow for correlations to be intrinsically described without any *a priori* requirements. Coherent systems (that is states whose one-body reduced density matrix has a single contributing eigenvalue) [8] and fragmented systems (that is states whose one-body reduced density matrix has several macroscopic eigenvalues) [9, 10] can be described by MCTDHB alike.

Notably, when $M = 1$ is set in Eq. (4) the MCTDHB ansatz becomes identical to the wavefunction ansatz of the time-dependent Gross-Pitaevskii (TDGP) theory and, consequently, the MCTDHB equations of motion boil down to the TDGP equation. For further details about the MCTDHB method see Refs. [1, 2, 11].

## S2. INTERWELL CORRELATION FOR CONTACT INTERACTION

The left-right inter-well correlation can be defined as:

$$|g^{(1)}(x_l, x_r)|^2 = \left| \frac{\rho^{(1)}(x_r, x_l;t)}{\sqrt{\rho^{(1)}(x_r, x_r;t)\rho^{(1)}(x_l, x_l;t)}} \right|^2. \tag{6}$$

The quantity $|g^{(1)}(x_l, x_r)|^2$ gives the degree of first-order correlation between points $x = x_r$ and $x' = x_l$. For our potential, Eq. (3), the position $x_r$ ($x_l$) of the right (left) well extends

from about 1.5 to 2.1 ($-1.5$ to $-2.1$) for the considered tilts $\alpha$. We therefore choose $x_l = -1.5$ and $x_r = 1.5$ and plot the inter-well correlations as a function of the tilt $\alpha$ for various barrier heights $V_0$ and interaction strengths $\lambda$ in Fig. S1.

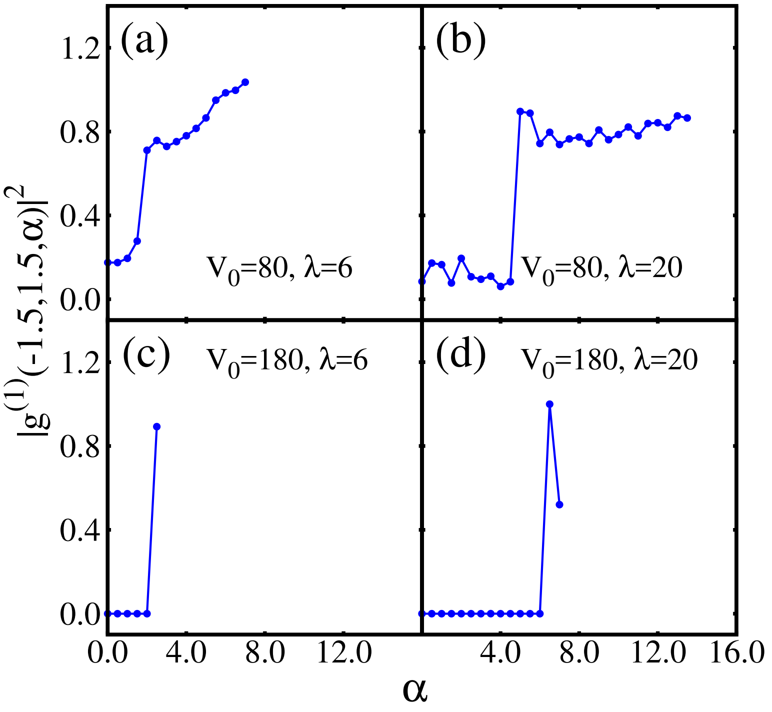


FIG. S1. Behavior of the first-order inter-well correlation function, $|g^{(1)}(x_l, x_r)|^2$, for varying barrier height and interaction strength for various values of $\alpha$. (a) and (b) correspond to $\lambda = 6$ and $\lambda = 20$ for $V_0 = 80$. We plot the correlations for values of $\alpha$ where the one-body density $\rho(x_{l,r})$ is larger than 0.01. Similarly (c) and (d) correspond to $\lambda = 6$ and $\lambda = 20$ for $V_0 = 180$. In this case the correlations of bosons in the outermost wells at $x_l = -1.5, x_r = 1.5$ are considered.

For moderate barrier height (and smaller interaction strength), inter-well correlation persists for a smaller $\alpha$ window. However, it disappears with a further increase of $\alpha$ at $\lambda = 6$ [see Fig. S1(a)]. Further increasing the interaction strength ($\lambda = 20$) leads to higher left-right correlation that is also increasing with $\alpha$ [Fig. S1(b)].

In the case of larger barrier height, the left-right correlation is observed only for certain values of the tilting parameter [Fig. S1(c) and (d)]. Hence, by tuning the barrier height, interaction strength and tilt of the well, the left-right coherence can be adjusted.

## S3. CONVERGENCE OF RESULTS WITH RESPECT TO THE NUMBER OF ORBITALS

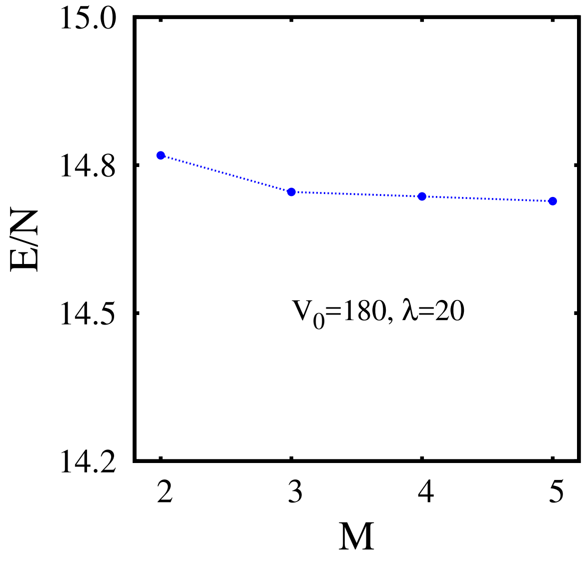


FIG. S2. Ground state energy per particle $E/N$ as a function of the number of orbitals $M$ for barrier height $V_0 = 180$ and $\lambda = 20$ for contact interactions. The energy converges for increasing $M$.

Fig. S2 shows the behavior of the ground state energy per particle $E/N$, for a fixed barrier height and interaction strength as the number of orbitals $M$ increases; $E/N$ drops at a decreasing rate demonstrating convergence. The same behavior is observed for $E/N$ for different values of the barrier height and interaction strengths. We conclude that the convergence of our results with respect to the number of orbitals is satisfactory.

## S4. NATURAL OCCUPATIONS AND FIRST-ORDER CORRELATION FUNCTION IN THE CASE OF LONG-RANGE INTERACTION

The long-range interaction of two bosons at $x_j$ and $x_k$, respectively, is assembled as [12–14]

$$\hat{W}(x_j - x_k) = \frac{\lambda_0}{|x_j - x_k|^3 + \Delta^3} \ , \tag{7}$$

where $\Delta^3 = 0.07$ is the threshold of the long-range interaction and $\lambda_0$ is the interaction strength [1, 15]. Such long-range interactions are relevant for atomic clouds made of Cr [16],

Dy [17] or Er [18].

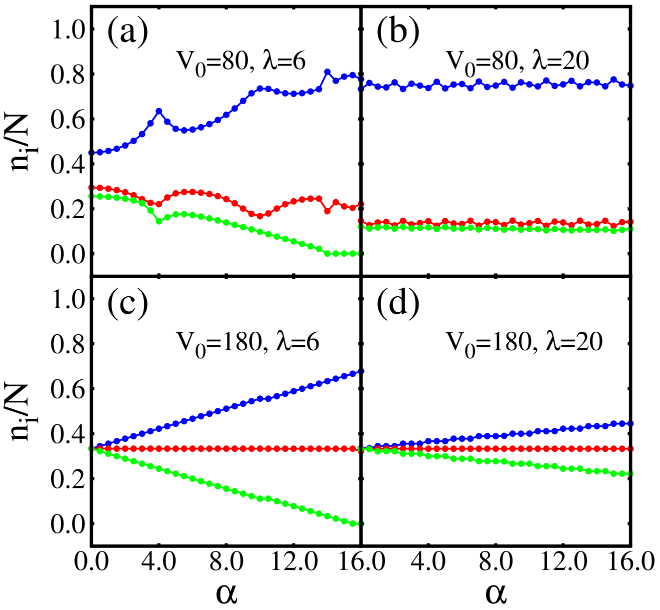


FIG. S3. This figure shows the variation of natural occupations, $n_i/N$ as a function of the tilt $\alpha$ for long-range interactions. (a) corresponds to $V_0 = 80$ and $\lambda = 6$, (b) corresponds to $V_0 = 80$ and $\lambda = 20$, (c) corresponds $V_0 = 180$ and $\lambda = 6$ and (d) corresponds $V_0 = 180$ and $\lambda = 20$. In all panels, blue lines with circles represents $n_1$, red lines with circles represents $n_2$ and green lines with circles represents $n_3$.

### A. Natural Occupations

Fig. S3 shows the behavior of the natural occupations $n_i/N$ as a function of the tilt parameter $\alpha$ for fixed barrier height $V_0$ and interaction strength $\lambda$, in the case of long-range interaction as given by Eq. (7). For the choices $V_0 = 80$, $\lambda = 6$ and zero tilt $\alpha = 0$ threefold fragmentation of the condensate is observed [Fig. S3(a)]. With the inclusion of the tilt $\alpha > 0$, there is a gradual increase in the value of the first natural occupation, $n_1/N$, and a decrease in the value of the second and the third natural occupations, $n_2/N$ and $n_3/N$. However, for a larger interaction strength, $\lambda = 20$, the occupations are unaffected from the tilt. This is due to the (surprising) fact that the zero-tilt strongly-interacting system exhibits very little fragmentation; increasing values of $\alpha$ do not alter this behavior [Fig. S3(b)].

For larger barrier height $V_0 = 180$ (and $\lambda = 6$), a completely threefold fragmented state

is observed for no tilt, $\alpha = 0$, see Fig. S3(c). For $\alpha > 0$, we see a gradual increase of the first natural occupation, $n_1/N$, and a corresponding decrease of the third natural occupation, $n_3/N$. However, the second natural occupation, $n_2/N$, remains constant irrespective of the increasing values of $\alpha$ (unlike in the case of contact interaction, cf. Fig. 2(c) in the main text).

For larger interaction strength, $\lambda = 20$, the system remains threefold fragmented up to a moderate value of $\alpha$ near $\alpha \sim 4$. With a further increase of $\alpha$, a very slow increase in $n_1/N$ and a corresponding slow decrease in $n_3/N$ are observed, while $n_2/N$ remains constant irrespective of the increase in $\alpha$. However, the state of the system is not settling back to fully condensed as $\alpha$ increases further [Fig. S3(d)] – at least for the tilts $\alpha \leq 16$ which we consider here.

We see that, generally, long-range interactions favor fragmentation in the condensate, compare Fig. S3 with Fig. 2 in the main text.

### B. First-order correlation function

To gain a spatially resolved picture of the fragmentation and coherence properties of the many-body state for the case of long-range interactions, we discuss the behavior of the first-order correlation function $|g^{(1)}(x'_1, x_1)|^2$. The latter is plotted for $\alpha = 15.2, 16$ and interaction strengths $\lambda = 6, 20$ for a large barrier height, $V_0 = 180$, in Fig. S4.

For $\lambda = 6$, an increase in the barrier height leads to the localization of the system. Similarly to the case of contact interactions studied in the main text (Fig. 3 and its discussion), a decrease in the coherence between bosons in distinct wells is observed as $\alpha$ grows. However, for some values of the tilt $\alpha$ the inter-well coherence between the bosons re-emerges, see Fig. S4(a). For large interaction strength, $\lambda = 20$, the coherence among bosons in distinct wells is lost irrespective of the increase in the values of $\alpha$ [panels (c)-(d) of Fig. S4]. As in the case of contact interactions in the main text, the barrier height can be used to quench the inter-well coherence also for long-ranged interactions. Moreover, the tilt can be used to tune the coherence between neighboring wells for long-ranged interactions, too.

---

[1] O. E. Alon, A. I. Streltsov, and L. S. Cederbaum, Phys. Rev. A **77**, 033613 (2008).

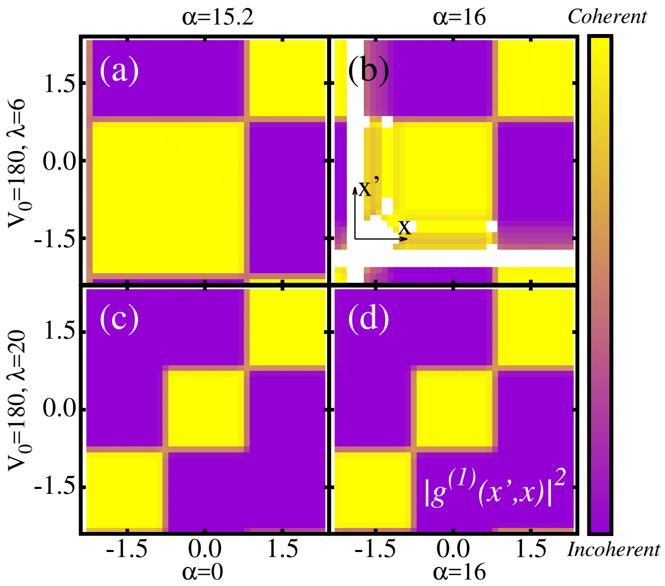


FIG. S4. The first-order correlation $|g^{(1)}(x_1', x_1)|^2$ is visualized as a function of the tilt and barrier height for $V_0 = 180$ in the case of long-range interaction. (a) and (b) correspond to $\alpha = 15.2$ and $\alpha = 16$ respectively for $\lambda = 6$. Similarly (c) and (d) correspond to $\alpha = 0$ and $\alpha = 16$ for $\lambda = 20$.


[2] A. U. J. Lode, Phys. Rev. A **93**, 063601 (2016).

[3] E. Fasshauer and A. U. J. Lode, Phys. Rev. A **93**, 033635 (2016).

[4] M. C. Tsatsos, J. H. V. Nguyen, A. U. J. Lode, G. D. Telles, D. Luo, V. S. Bagnato, R. G. Hulet, arXiv:1707.04055 (2017).

[5] *Geometry of the time-dependent variational principle*, P. Kramer and M. Saracen, (Springer, Berlin, 1981).

[6] A. U. J. Lode, *Tunneling Dynamics in Open Ultracold Bosonic Systems*, Springer Theses, (Springer, Heidelberg, 2014).

[7] A. U. J. Lode, K. Sakmann, O. E. Alon, L. S. Cederbaum, and A. I. Streltsov, Phys. Rev. A 86, 063606 (2012).

[8] O. Penrose and L. Onsager, Phys.Rev. **104**, 576 (1956).

[9] P. Nozières, D. Saint James, J. Phys. (France) **43**, 1133 (1982).

[10] R. W. Spekkens and J. E. Sipe, Phys. Rev. A **59**, 3868 (1999).

[11] A. I. Streltsov, O. E. Alon, and L. S. Cederbaum, Phys. Rev. Lett. **99**, 030402 (2007).

[12] S. Zöllner, G. M. Bruun, C. J. Pethick, and S. M. Reimann, Phys. Rev. Lett. **107**, 035301 (2011).

[13] S. Zöllner, Phys. Rev. A **84**, 063619 (2011).

[14] U. R. Fischer, A. U. J. Lode, and B. Chatterjee, Phys. Rev. A **91**, 063621 (2015).

[15] *Many-body Schrödinger dynamics of Bose-Einstein condensates*, Kaspar Sakmann, (Springer, 2011).

[16] A. Griesmaier, J. Werner, S. Hensler, J. Stuhler, and T. Pfau, Phys. Rev. Lett. **94**, 160401 (2005).

[17] M. Lu, N. Q. Burdick, S. H. Youn, and B. L. Lev, Phys. Rev. Lett. **107**, 190401 (2011).

[18] K. Aikawa, A. Frisch, M. Mark, S. Baier, A. Rietzler, R. Grimm, and F. Ferlaino, Phys. Rev. Lett. **108**, 210401 (2012).
